# Supplementary material for: Private DNA Sequencing: Hiding Information in Discrete Noise
Source: arXiv:2101.12124 source file (2024-11-04)
Supplement: Supplementary file 1 [file additional_results.tex]

\section{Additional Comments}

\begin{lemma} 
	For any $K \in \mathbb{N}, p \in [0, 0.5],$ we have that 
	\begin{align} 
	& I(X \; ; \; X + \sum_{i=1}^K Y_i) \\
	& = H(p) - \sum_{i=0}^{K-1} p^{K-i} (1-p)^{i+1} \binom{K+1}{i+1} H \left(\frac{i+1}{K+1}\right).
	\end{align}
\end{lemma}

\begin{lemma}
	For any $K \in \mathbb{N},$  $p = c(1 - e^{-\frac{1}{K+1}}),$ and $L \in \mathbb{N}$ such that $L \leq K$ and $c \in \mathbb{R}, \; \; 0 \leq c \leq 1,$ we have that 
	\begin{align} 
	& I(X \; ; \; X + \sum_{i=1}^K Y_i)
	\\ & \leq c \left( \frac{1}{K+1} \right) \log\left(c \left(K+2 \right) \right) 
	\\ & + \left( \frac{K+2-c}{K+2} \right) \log\left(\frac{K+1}{K+1-c} \right)
	\\ & - c\left( \frac{K-L+2}{K+2} \right)^{L} \left( \frac{1}{K+1} \right) \log \left( \frac{K+1}{L} \right) 
	\\ & \times \left(1 - \frac{c}{K+1} \right)^{K} e^c \left(1 - \frac{1}{\sqrt{2 \pi L}}  \left(\frac{ce}{L}\right)^L \right)   
	\end{align}
\end{lemma}

Substituting $L = \ln(K)$ into the bound above, we have that 

Thus, the perfomance of the uniform scheme is upper bounded by  
\begin{align}
&  c \left( \frac{1}{K+1} \right) \log\left(c \left(K+2 \right) \right) 
\\ & + \left( \frac{K+2-c}{K+2} \right) \log\left(\frac{K+1}{K+1-c} \right)
\\ & - c\left( \frac{K-\ln(K)+2}{K+2} \right)^{\ln(K)} \left( \frac{1}{K+1} \right) \log \left( \frac{K+1}{\ln(K)} \right) 
\\ & \left(1 - \frac{c}{K+1} \right)^{K} e^c \left(1 - \frac{1}{\sqrt{2 \pi \ln(K)}}  \left(\frac{ce}{\ln(K)}\right)^{\ln(K)} \right)  
\\ & \sim \frac{c\ln(\ln(K))}{\ln(2)K}
\end{align}

We also have the lower bound at $p = c (1 - e^{-\frac{1}{K+1}})$ is given by 
\begin{align}
& -\left(1 - c(1 - e^{-\frac{1}{K+1}}) \right)^{K+1} \log(1 - c(1 - e^{-\frac{1}{K+1}}))
\\ & - \left(1 - c(1 - e^{-\frac{1}{K+1}}) \right)^{K+1} \log(1 - (1 - c(1 - e^{-\frac{1}{K+1}}))^K)
\\ & + \left(1 - c(1 - e^{-\frac{1}{K+1}}) \right)^{K+1} \log(1 - (1 - c(1 - e^{-\frac{1}{K+1}}))^{K+1})
\\ & + \left(1 - c(1 - e^{-\frac{1}{K+1}}) \right) \log(1 - \left(1 - c \left(1 - e^{-\frac{1}{K+1}} \right) \right)^{K})
\\ & -\log(1 - (1 - c(1 - e^{-\frac{1}{K+1}}))^{K+1})
\\ & \sim \frac{c e^{-c}}{K \ln(2)}
\\ & - \frac{(c-3)c e^{-c}}{2(e^c-1)K \ln(2)} + \frac{(c-1)c e^{-c} \ln(1 - e^{-c})}{2K \ln(2)} 
\\ & + \frac{(c-1)c e^{-c}}{2(e^c-1)K \ln(2)}  - \frac{(c-1)c e^{-c} \ln(1-e^{-c})}{2K \ln(2)} 
\\ & - \frac{c \ln(1 - e^{-c})}{K \ln(2)}  + \frac{(c-3)c}{2(e^c-1)K \ln(2)}
\\ & - \frac{(c-1)c}{2(e^c-1)K \ln(2)}
\\ & = \Theta \left( \frac{1}{K} \right)
\end{align}

This proves that the ratio between the performance of the uniform scheme and the lower bound for $p = c(1 - e^{-\frac{1}{K+1}})$ is upper bounded by a function that is $O(\ln(\ln(K)))$ for $0 \leq c \leq 1.$
