# Supplementary material for: Private DNA Sequencing: Hiding Information in Discrete Noise
Source: arXiv:2101.12124 source file (2024-11-04)
Supplement: Supplementary file 2 [file appendix_proofs10_19_20.tex]

\begin{lemma}
    \label{lem:alpha0_condition}
    Fixing $\alpha_0 = 1$ in the optimization problem (\ref{eq:integral_alpha_opt_prob}) does not change the optimal value.
\end{lemma}

\begin{IEEEproof}
    Let $\alpha_0 \in \mathbb{N}.$ 
	Let $Z$ be any random variable such that its pmf has integral support and maximum support value at $t = 0.$  Let 
	\begin{align}
	& \hat{Z} = Z - S
	\end{align} 
	where $S = Z \mod{\alpha_0}.$ 
	We then have that 
	\begin{align}
	& I(X ; \alpha_0 X + 	Z)  \geq I(X ; \alpha_0 X + \hat{Z}).   
	\end{align} 
	because
	\begin{align} 
		& I(X ; \; \alpha_0 X + 	Z)
		\nonumber \\ & = I(X ; \; \alpha_0 X + \hat{Z} +  S)
		\nonumber \\ & = I(X ; \; \alpha_0 X + \hat{Z}, \; S)
		\nonumber \\ & = I(X ; \; S) + I(X ; \; \alpha_0 X + \hat{Z} \; | \; S)
		\nonumber \\ & = I(X ; \; \alpha_0 X + \hat{Z} \; | \; S)
		\nonumber \\ & = H(X \; | \; S)  - H(X \; | \; \alpha_0 X + \hat{Z}, \; S) 
		\nonumber \\ & = H(X)  - H(X \; | \; \alpha_0 X + \hat{Z}, \; S)
		\nonumber \\ & \geq H(X)  - H(X \; | \; \alpha_0 X + \hat{Z})
		\nonumber \\ & = I(X \; ; \; \alpha_0 X + \hat{Z})
	\end{align} 
	where the third line follows because given $\alpha_0 X + \hat{Z} + S,$ we have that 
	\begin{align}
	    S = ((\alpha_0 X + \hat{Z} + S) - \alpha_0) \mod  \alpha_0 
	\end{align}
	and
    \begin{align}
	    \alpha_0 X + \hat{Z} = (\alpha_0 X + \hat{Z} + S) - S.
	\end{align}
	Thus, any solution to (\ref{eq:relax_inf1}) with  $\alpha_0 = a$ can be transformed into a solution whose pmf had support values in $\{t a : \; t \in \mathbb{Z}\}$ without increasing the mutual information.   Therefore, for a fixed $\alpha_0,$ it suffices to only consider pmfs that have support values in $\{t \alpha_0 : \; t \in \mathbb{Z}\}$ in the optimization.  If $\alpha_0 = a ,$ any solution random variable $D$ with  support values in $\{t a : \; t \in \mathbb{Z}\}$ can be transformed into a solution with the same mutual information, $\alpha_0 = 1,$ and support values in $\{t : \; t \in \mathbb{Z}\}.$ This is accomplished by dividing $D$ by $a.$  Therefore it suffices to fix $\alpha_0=1$ in the optimization. 
\end{IEEEproof}
	
	\begin{lemma}
	\label{lem:solve_KKT}
	    A solution to problem (\ref{eq:relax_const_pert_posq}) is given by
	   % (\ref{eq:KKT_conditions_sol})
\begin{align}
\label{eq:KKT_conditions_sol_full}
& q_{(-i)} =  \beta (1 - \beta)^{i}  \text{ for } i \in \{0,...,n+1\} 
\nonumber \\ & v_1 = - p \log \left( \frac{p}{(1-p)(1 - \beta) + p} \right) 
\nonumber \\ & \quad - (1-p)\log \left( \frac{(1-p)(1 - \beta)}{(1-p)(1 - \beta) + p} \right)
\nonumber \\ & v_2 = (1-p)\log \left( \frac{(1-p)(1 - \beta)}{(1-p)(1 - \beta) + p} \right) 
\nonumber \\ & v_3 = p \log \left( \frac{p}{(1-p)(1 - \beta) + p} \right).
\end{align}
	\end{lemma}
	\begin{IEEEproof}
	Let $f_0(q)$ be the objective function of (\ref{eq:relax_const_pert_posq}).  
% 	The Lagrangian is given by 
% 	\begin{align} 
% 	&L(q, v, \lambda) = f_0(q) 
% 	\nonumber \\ & + v_1 \left(\sum_i q_{(i)} - 1 + (1 - (1-p)^K)^{n+2} \right) 
% 	\nonumber \\ & + v_2 \left(q_{(0)} - (1-p)^K \right) 
% 	\nonumber \\ & + v_3 \left(q_{(-n-1)} - (1-p)^K (1 - (1-p)^K)^{n+1} \right). 
% 	\end{align}
	The Lagrangian of (\ref{eq:relax_const_pert_posq}) is given in (\ref{eq:lagrangian}).
	The derivative of $f_0(q)$ with respect to $q_{(j)}$ is given by 
	\begin{align}
	& p \log \left(\frac{p q_{(j)}}{(1-p)q_{(j-1)} + p q_{(j)}} \right) \nonumber \\ & + (1-p) \log \left( \frac{(1-p) q_{(j)}}{p q_{(j+1)} + (1-p) q_{(j)}} \right)
	\end{align}  
	for $j \in \{-n, \; ..., \;  -1\}$ and the KKT conditions are given by 
	\begin{align}
	& q_{(0)} = (1-p)^K,
	\nonumber \\ & q_{(-n-1)} = (1-p)^K (1 - (1-p)^K)^{n+1}, 
	\nonumber \\ &     \sum_{j} q_{(j)} = 1 - (1 - (1-p)^K)^{n+2}
	\nonumber \\ & (1-p) \log \left( \frac{(1-p) q_{(j)}}{p q_{(j+1)} + (1-p) q_{(j)}} \right) + v_1 + v_3 = 0 \quad 
	\nonumber \\ &  \text{for } j = - n -1
	\nonumber \\ & 	p \log \left(\frac{p q_{(j)}}{(1-p)q_{(j-1)} + p q_{(j)}} \right) 
	\nonumber \\ & + (1-p) \log \left( \frac{(1-p) q_{(j)}}{p q_{(j+1)} + (1-p) q_{(j)}} \right)+ v_1 = 0 
	\nonumber \\ &  \forall j \in \{-n, \; ..., \;  -1\}
	\nonumber \\ & p \log \left(\frac{p q_{(j)}}{(1-p)q_{(j-1)} + p q_{(j)}} \right) + v_1 + v_2 = 0 
	\nonumber \\ & \text{for } j = 0.
	\end{align}

	The last three conditions can be rewritten as 
	\begin{align} 
	& (1-p) \log \left( \frac{(1-p) }{p \frac{q_{(j+1)}}{q_{(j)}} + (1-p) } \right) + v_1 + v_3 = 0  
	\nonumber \\ &  \text{for } j = - n - 1
	\nonumber \\ & p \log \left(\frac{p }{(1-p)\frac{q_{(j-1)}}{q_{(j)}} + p } \right) \nonumber \\ & + (1-p) \log \left( \frac{(1-p) }{p \frac{q_{(j+1)}}{q_{(j)}} + (1-p) } \right)   + v_1  = 0 
	\nonumber \\ & \forall j \in \{-n, \; ..., \;  -1\}
	\nonumber \\ & p \log \left(\frac{p }{(1-p) \frac{q_{(j-1)}}{q_{(j)}} + p } \right)  + v_1 + v_2  = 0 \quad \text{for } j = 0
	\end{align}
	which shows that if the ratio $\frac{q_{(j-1)}}{q_{(j)}}$ between consecutive variables is the same for all $j,$  then $v_1,$ $v_2$ can  be chosen so that of these derivatives equal $0$ for all $j.$  Picking \[\frac{q_{(j-1)}}{q_{(j)}} = (1 - (1-p)^K),\] a solution to these equations is then
	\begin{align}
	& q_{(-i)} =  (1-p)^K (1 - (1-p)^K)^{i}  
	\nonumber \\ & \text{for } i \in \{0, \; 1, \; ..., \; n+1 \} 
	\nonumber \\ & v_1 = - p \log \left( \frac{p}{(1-p)(1 - (1-p)^K) + p} \right) 
	\nonumber \\ & - (1-p)\log \left( \frac{(1-p)(1 - (1-p)^K)}{(1-p)(1 - (1-p)^K) + p} \right)
	\nonumber \\ & v_2 = (1-p)\log \left( \frac{(1-p)(1 - (1-p)^K)}{(1-p)(1 - (1-p)^K) + p} \right) 
	\nonumber \\ & v_3 = p \log \left( \frac{p}{(1-p)(1 - (1-p)^K) + p} \right).
	\end{align}
	\end{IEEEproof}
	
	\rdcomment{this may be similar to the IS comments, but this proof is a bit hard to read for me. i understand the first few paragraphs in words, but it is not trivial to me to see exactly how this formally changes the problem. i would suggest stating the problem, and then how the support-constraint changes the optimization, and so on. to be honest, if you're tight on space, i still think it would be more beneficial to dedicate more space to this `reduction' and then even leave some of the more mechanical parts of derivatives/KKT condition analysis out.

also, we arrived at this result through figures and drawings; can we add some of this into the proof? i think it would strengthen the appeal of this paper to hint at why the idea is actually intuitive and cute. as written, it feels more a set of mechanical manipulations of KKT conditions, and it loses the sort of elegance i typically associate with info theory papers. (this is not a comment on the result, it's just a comment on the presentation and how it makes me feel.) i really liked the drawings of the convolution of discrete measures, and how we're really chosing a measure that gets shifted to the left by 1 and rescaled by 1-p and shifted to the right by 1 and rescaled by p. can this be put in this section at all?}

\rdcomment{stupid question: can you tell me a little more why (12) is this derivative? at a glance, it seems to be that there's a ton of term cancellations... (it's like the terms inside the log don't depend on $q_j$ with the way the derivative is written, so all those terms cancel?) i fear that a unfastidious reviewer may just claim this is a fundamental error and give a poor review without analyzing it deeply. (this happens sometimes to me.)}
